# Supplementary material for: Efficient Hyperparameter Optimization for Physics-based Character Animation
Source: arXiv:2104.12365 source file (2021-04-26)
Supplement: Supplementary file 1 [file appendix.tex]

% \section{Bayesian Optimization}

% \begin{figure*}[h]
%   \centering
%   \includegraphics[width=\linewidth]{img/bo.pdf}
%   \caption{\zeshi{An example of the BO optimization process applied to a one-dimensional function. The green dotted curve represents the unknown black-box function. The red curve and points indicate the predicted mean values and sampled points respectively. The rosy region shows estimated uncertainty, $95\%$ confidence intervals. The blue curve is the acquisition function that is maximized to select the next sample point (It is scaled for the convenience of visualization). The blue downside arrows indicate the selected point in the next iteration.}}
%   \label{fig:BO}
% \end{figure*}


% \zeshi{Given a black-box function $f(x)$, where $x$ is the input hyperparameter from a $d$-dimensional bounded space $\mathcal{A}$, BO aims to find the optimum of the function, $x^{\star}$ with the number of necessary evaluations as small as possible. Suppose we currently have a set of observations $D_{t} = \{(x_{i}, y_{i})\}_{i=1}^{i=t}$, where $y_{i}$ is a noisy measurement of $f(x_{i})$. We want to select the next sampling point based on previous observations. The \textit{acquisition function} $a: \mathcal{A} \to \mathbb{R}$ is a function quantifying the utility of any arbitrary sampling candidates. The next sampling point is obtained by maximizing the acquisition function:
% \begin{equation}
%     x_{t+1} = \mathop{\arg\max}\limits_{x \in \mathcal{A}}a(x, D_{t})
% \end{equation}}

% \zeshi{The acquisition function is designed with consideration  for both finding candidate parameters with large values and making evaluations more informative. Querying a sampling point close to already visited points is less informative. Gaussian Process Upper Confidence Bound (GP-UCB) \cite{srinivas2010gaussian} is a popular choice for the acquisition function. It is defined as:
% \begin{equation}
%     a(x, D_{t}) = \mu_{t}(x) + \beta^{\frac{1}{2}} \sigma_{t}(x)
% \end{equation}
% where $\mu_{t}(x)$ and $\sigma_{t}(x)$ are approximated posterior mean value and standard deviation of $f(x)$ respectively.
% $\mu_{t}(\cdot)$ favours candidates which are likely to have large values. $\sigma_{t}(\cdot)$ encourages to query points whose uncertainty is high. $\beta$ enables a trade-off between exploitation and exploration.}

% \zeshi{Computing $\mu_{t}(\cdot)$ and $\sigma_{t}(\cdot)$ in closed forms are available by assuming gaussian prior on $f(\cdot)$: any finite set of values of evaluations follow a multivariate gaussian distribution. Gaussian Process (GP) \cite{rasmussen2003gaussian} is a common choice of surrogate model for modelling functions. It contains a prior mean function $m(x)$ and a kernel function $k(x,x')$. $m(x)$ encodes our prior belief of the objective function's mean values. The kernel function $k(x,x')$ measures correlations between $f(x)$ and $f(x')$. Given $m(\cdot)$, $k(\cdot, \cdot)$ and previous observations $D_{t}$, $\mu_{t}$ and $\sigma_{t}$ could be computed in closed forms:
% \begin{equation}
%     \begin{gathered}
%         \mu_{t}(x) = k(x,X) (K + \eta^{2} I)^{-1} Y \\
%         \sigma_{t}^{2}(x) = k(x, x) + \eta^{2} - k(x,X)(K + \eta^{2}I)^{-1} k(X,x)
%     \end{gathered}
% \end{equation}
% where $Y \in \mathbb{R}^{t}, Y_{i} = y_{i}$; $X \in \mathbb{R}^{t \times d}, X_{i} = x_{i} $; $K \in \mathbb{R}^{t \times t}, K_{i,j} = k(x_{i}, x_{j})$; $k(x,X) = (k(x,x_{1}),k(x,x_{2}),...k(x,x_{t}))$. $\eta$ is the standard deviation of the observation noise.}

% \zeshi{Many choices of kernel functions exist, including Square Exponential kernel and Matern kernel. In this work we adopt the Square Exponential kernel defined as:
% \begin{equation}
%     k_{SE}(x, x') = \sigma_{f}^{2}  exp(-\frac{1}{2}(x-x')^{T}\Lambda^{-1}(x-x'))
% \end{equation}
% $\Lambda = diag(\lambda_{1}, \lambda_{2},...\lambda{t})$, where $\lambda_{i}$ is the length scale of the i-th component of inputs. $f(\cdot)$ is flat across the i-th component of inputs when $\lambda_{i}$ is large.}

% \zeshi{Figure \ref{fig:BO} shows optimization sequences of BO on a one-dimensional function. For more details, we refer readers to the second chapter of \cite{rasmussen2003gaussian}.}

% \section{Deep Reinforcement Learning}
% \zeshi{The policy learning of simulated agents could be formulated as a standard reinforcement learning problem: where agents interact with the environment to maximize expected rewards using optimized policies. The control policy $\pi_{\theta}(a_{t}|s_{t})$ models the conditional distribution of action $a_{t}$ given the agent's current state $s_{t}$. The agent takes action $a_{t}$, gets reward $r_{t}$ and then transits to next state $s_{t+1}$ according to probabilistic environment dynamics $p(s_{t+1}|a_{t}, s_{t})$. The goal is to learn the optimal policy $\pi_{\theta^{\star}}$ to maximize the expected return:
% \begin{equation}
%     J(\theta) = \mathbb{E}_{\pi_{\theta}}[\sum_{t=0}^{T}\gamma^{t}r_{t}]
% \end{equation}
% where $T$ is the episode length and $\gamma$ is the discount factor.}

% \zeshi{One popular class of reinforcement learning algorithm is policy gradient methods\cite{sutton2000policy}. The gradient of the expected return $\nabla_{\theta}J(\theta)$ is given by:
% \begin{equation}
%     \nabla_{\theta}J(\theta) = \mathbb{E}_{\pi_{\theta}}[\nabla_{\theta}log \pi_{\theta}(a_{t}|s_{t})A_{t}]
% \end{equation}
% where $A_{t}$ is the advantage function which is defined as
% \begin{equation}
%     A_{t} = \sum_{l = 0}^{T-t}\gamma^{l}r_{t+l} - V(s_{t})
% \end{equation}
% $\sum_{l = 0}^{T-t}\gamma^{l}r_{t+l}$ denotes the return when taking the action $a_{t}$ given state $s_{t}$. $V(s_{t})$ represents the value function which computes the expected return of state $s_{t}$ by following current policy. A straightforward understanding of policy gradient methods is to increase the likelihood of actions which get high returns and decrease the likelihood of taking undesirable actions.
% }

% \zeshi{In this work, we use Proximal Policy Optimization (PPO) \cite{schulman2017proximal} to train control policies, a frequently used on-policy DRL algorithms for physics-based character control. $TD(\lambda)$ is used to compute the value function. Advantage functions are computed by using generalized advantage estimation $GAE(\lambda)$ \cite{schulman2015trust}.}
